# Supplementary material for: Observations of cold gas and star formation in dwarf S0 galaxies
Source: arXiv:2108.09705 source file (2021-08-22)
Supplement: Supplementary file 1 [file appendix.tex]

\begin{table*}
    \begin{threeparttable}
        \centering
      \caption{
        List of telluric lines used in this work, compiled as described in Section \ref{sec:tellines},
        including their wavelengths and depths relative to a normalised continuum of 1.
    }
\begin{tabular}{p{1cm}p{1.5cm}|p{1cm}p{1.5cm}|p{1cm}p{1.5cm}|p{1cm}p{1.5cm}|p{1cm}p{1.5cm}}
        \toprule
      $\lambda$, \AA & Depth, \% &       $\lambda$, \AA & Depth, \% &       $\lambda$, \AA & Depth, \% &       $\lambda$, \AA & Depth, \% &       $\lambda$, \AA & Depth, \% \\
        \midrule
5030.14 & 2.12 & 5457.11 & 2.60 & 5883.60 & 4.45 & 5908.07 & 5.52 & 5941.22 & 8.60  \\
5035.19 & 2.12 & 5463.17 & 2.49 & 5883.78 & 3.05 & 5908.17 & 2.57 & 5941.67 & 3.84  \\
5035.21 & 2.32 & 5682.53 & 2.16 & 5883.82 & 3.08 & 5908.27 & 2.67 & 5941.88 & 23.47  \\
5035.36 & 2.37 & 5684.57 & 2.29 & 5883.87 & 2.28 & 5908.63 & 6.40 & 5942.00 & 2.87  \\
5035.94 & 2.16 & 5684.63 & 3.49 & 5884.69 & 13.18 & 5909.00 & 6.31 & 5942.05 & 2.99  \\
5036.09 & 2.16 & 5686.19 & 3.12 & 5885.00 & 3.35 & 5909.79 & 13.05 & 5942.43 & 17.72  \\
5036.40 & 2.99 & 5688.24 & 6.68 & 5886.44 & 3.25 & 5910.25 & 2.33 & 5943.07 & 2.12  \\
5036.44 & 2.39 & 5690.35 & 3.61 & 5886.77 & 19.79 & 5910.99 & 5.76 & 5943.10 & 2.06  \\
5037.99 & 5.34 & 5691.20 & 4.74 & 5887.13 & 7.36 & 5911.08 & 2.33 & 5943.22 & 11.39  \\
5038.42 & 5.16 & 5693.19 & 6.07 & 5887.47 & 4.02 & 5911.12 & 2.07 & 5943.37 & 22.36  \\
5038.96 & 2.38 & 5696.72 & 2.14 & 5888.02 & 16.30 & 5911.28 & 2.09 & 5945.12 & 10.26  \\
5038.98 & 2.37 & 5698.94 & 4.39 & 5888.45 & 12.91 & 5911.44 & 2.51 & 5945.54 & 8.39  \\
5039.54 & 2.06 & 5700.09 & 4.90 & 5888.65 & 2.56 & 5911.56 & 10.93 & 5946.08 & 4.62  \\
5042.08 & 2.22 & 5701.49 & 5.53 & 5889.51 & 8.52 & 5912.81 & 2.14 & 5946.10 & 4.75  \\
5042.58 & 3.01 & 5712.15 & 2.03 & 5890.43 & 14.86 & 5913.49 & 3.45 & 5946.45 & 8.47  \\
5042.80 & 2.32 & 5718.27 & 3.49 & 5890.88 & 13.39 & 5913.79 & 11.13 & 5946.81 & 20.56  \\
5043.59 & 3.04 & 5719.71 & 2.44 & 5891.00 & 3.11 & 5914.99 & 8.47 & 5947.65 & 10.54  \\
5043.77 & 4.25 & 5720.34 & 4.84 & 5891.94 & 3.19 & 5915.73 & 5.90 & 5947.86 & 18.67  \\
5044.64 & 4.07 & 5722.70 & 2.87 & 5892.28 & 4.57 & 5916.23 & 7.33 & 5949.01 & 2.40  \\
5053.06 & 2.57 & 5722.73 & 2.97 & 5892.45 & 19.40 & 5916.42 & 6.26 & 5949.03 & 2.46  \\
5053.08 & 2.39 & 5724.66 & 2.40 & 5893.19 & 14.27 & 5917.37 & 3.19 & 5949.56 & 2.89  \\
5057.09 & 2.85 & 5727.64 & 3.76 & 5893.84 & 7.46 & 5917.39 & 3.15 & 5949.98 & 17.82  \\
5057.12 & 3.81 & 5730.44 & 3.43 & 5894.30 & 7.48 & 5918.19 & 3.63 & 5950.47 & 2.24  \\
5058.27 & 5.78 & 5736.33 & 2.47 & 5895.18 & 4.93 & 5919.22 & 15.37 & 5950.62 & 7.34  \\
5058.91 & 2.37 & 5738.45 & 5.32 & 5895.75 & 4.22 & 5919.85 & 20.91 & 5950.95 & 2.36  \\
5058.93 & 2.31 & 5742.98 & 3.02 & 5895.91 & 3.10 & 5920.44 & 26.24 & 5951.14 & 5.91  \\
5060.69 & 3.91 & 5746.56 & 4.47 & 5895.93 & 2.95 & 5921.36 & 7.89 & 5951.77 & 2.48  \\
5066.59 & 2.70 & 5754.98 & 2.40 & 5897.28 & 7.47 & 5921.96 & 2.34 & 5952.30 & 6.96  \\
5066.63 & 4.65 & 5755.02 & 2.11 & 5897.63 & 10.41 & 5923.16 & 3.20 & 5955.76 & 10.54  \\
5067.75 & 2.29 & 5762.38 & 2.05 & 5898.25 & 5.24 & 5923.31 & 11.64 & 5957.16 & 5.84  \\
5067.88 & 4.17 & 5764.17 & 2.14 & 5898.73 & 2.66 & 5923.51 & 3.36 & 5957.58 & 4.12  \\
5072.91 & 2.00 & 5860.39 & 2.33 & 5898.95 & 19.89 & 5923.98 & 2.47 & 5958.69 & 13.98  \\
5073.56 & 5.12 & 5860.43 & 2.10 & 5899.80 & 10.22 & 5924.44 & 10.02 & 5959.06 & 8.93  \\
5077.15 & 4.20 & 5871.43 & 3.98 & 5900.72 & 9.82 & 5924.63 & 13.14 & 5959.44 & 12.56  \\
5078.13 & 2.45 & 5872.08 & 2.25 & 5900.83 & 20.36 & 5925.07 & 18.02 & 5960.79 & 3.60  \\
5079.22 & 2.05 & 5876.38 & 3.45 & 5901.71 & 2.94 & 5925.79 & 10.78 & 5962.25 & 2.89  \\
5079.76 & 2.04 & 5876.91 & 5.43 & 5902.03 & 3.98 & 5929.09 & 11.76 & 5963.27 & 5.90  \\
5079.80 & 3.96 & 5877.24 & 4.04 & 5902.26 & 26.44 & 5929.92 & 2.80 & 5965.74 & 2.28  \\
5084.49 & 2.66 & 5880.39 & 4.82 & 5902.93 & 6.63 & 5931.41 & 2.10 & 5965.76 & 2.28  \\
5087.03 & 2.12 & 5880.51 & 5.27 & 5904.33 & 6.40 & 5932.89 & 18.87 & 5967.14 & 3.86  \\
5087.29 & 2.23 & 5881.51 & 3.07 & 5904.65 & 2.29 & 5933.58 & 11.01 & 5967.47 & 10.04  \\
5087.32 & 2.68 & 5881.54 & 2.92 & 5904.67 & 2.32 & 5934.88 & 2.63 & 5968.12 & 2.21  \\
5413.83 & 2.23 & 5881.73 & 5.29 & 5905.91 & 2.62 & 5935.99 & 2.20 & 5968.47 & 2.49  \\
5415.09 & 3.20 & 5881.89 & 4.12 & 5906.09 & 4.50 & 5936.61 & 6.16 & 5968.64 & 11.56  \\
5423.68 & 2.39 & 5882.66 & 5.73 & 5906.12 & 3.91 & 5938.85 & 4.90 & 5968.85 & 2.11  \\
5436.32 & 2.32 & 5882.77 & 4.44 & 5906.15 & 3.09 & 5940.76 & 3.37 & 5969.08 & 12.83  \\            \bottomrule
        \end{tabular}
    \end{threeparttable}
\end{table*}
\begin{table*}
    \begin{threeparttable}
        \centering
        \caption[]{
            \textit{(continued)} List of telluric lines used in this work.
        }
        \label{tab:actlines}
\begin{tabular}{p{1cm}p{1.5cm}|p{1cm}p{1.5cm}|p{1cm}p{1.5cm}|p{1cm}p{1.5cm}|p{1cm}p{1.5cm}}
            \toprule
$\lambda$, \AA & Depth, \% & $\lambda$, \AA & Depth, \% & $\lambda$, \AA & Depth, \% & $\lambda$, \AA & Depth, \% & $\lambda$, \AA & Depth, \%  \\
            \midrule \raggedright
5969.20 & 2.46 & 6282.80 & 25.81 & 6347.85 & 3.21 & 6481.10 & 2.08 & 6534.90 & 9.87  \\
5969.84 & 5.77 & 6283.35 & 3.82 & 6347.89 & 2.63 & 6482.53 & 4.12 & 6535.14 & 2.38  \\
5970.86 & 7.39 & 6283.57 & 20.67 & 6351.56 & 3.32 & 6484.11 & 22.67 & 6535.53 & 2.92  \\
5972.15 & 11.00 & 6284.64 & 16.35 & 6351.58 & 3.13 & 6484.55 & 2.32 & 6535.88 & 2.40  \\
5975.90 & 9.57 & 6285.38 & 8.22 & 6362.10 & 3.23 & 6484.63 & 7.53 & 6537.60 & 6.32  \\
5975.92 & 9.72 & 6286.65 & 6.62 & 6372.44 & 2.11 & 6484.79 & 11.07 & 6541.32 & 2.50  \\
5975.99 & 5.61 & 6288.60 & 14.60 & 6425.79 & 2.89 & 6485.53 & 4.52 & 6543.19 & 9.72  \\
5977.33 & 3.40 & 6289.99 & 2.31 & 6433.82 & 2.64 & 6486.43 & 5.92 & 6544.79 & 26.16  \\
5977.84 & 10.28 & 6290.25 & 18.17 & 6435.42 & 2.47 & 6486.53 & 2.53 & 6544.93 & 2.21  \\
5978.26 & 2.46 & 6291.07 & 24.21 & 6448.79 & 2.82 & 6487.65 & 12.62 & 6546.65 & 4.07  \\
5978.60 & 6.42 & 6291.69 & 2.29 & 6455.02 & 4.12 & 6488.42 & 2.31 & 6548.58 & 11.76  \\
5980.96 & 2.63 & 6293.01 & 25.49 & 6459.74 & 8.11 & 6488.90 & 4.21 & 6549.50 & 19.84  \\
5982.02 & 3.00 & 6293.46 & 5.67 & 6460.55 & 4.15 & 6490.01 & 8.24 & 6552.93 & 2.76  \\
5986.03 & 6.94 & 6293.81 & 30.05 & 6460.86 & 2.41 & 6491.66 & 25.31 & 6553.51 & 22.25  \\
5987.82 & 3.21 & 6295.48 & 3.33 & 6461.08 & 2.20 & 6491.82 & 2.18 & 6553.68 & 2.08  \\
5987.84 & 3.36 & 6295.51 & 3.44 & 6462.69 & 3.08 & 6493.79 & 17.40 & 6554.67 & 8.21  \\
5989.36 & 4.37 & 6296.03 & 28.03 & 6462.71 & 3.80 & 6494.11 & 6.00 & 6558.06 & 13.54  \\
5990.10 & 5.44 & 6296.81 & 32.24 & 6462.73 & 3.77 & 6495.29 & 4.75 & 6559.03 & 6.21  \\
5991.42 & 2.58 & 6298.11 & 5.95 & 6462.86 & 2.72 & 6496.74 & 25.31 & 6561.38 & 6.51  \\
5991.66 & 6.58 & 6299.31 & 28.31 & 6462.89 & 2.82 & 6498.37 & 2.97 & 6561.98 & 4.64  \\
5992.81 & 6.28 & 6300.08 & 31.46 & 6464.35 & 6.00 & 6498.48 & 6.83 & 6563.33 & 2.50  \\
5995.33 & 4.04 & 6302.85 & 25.46 & 6464.65 & 2.05 & 6503.46 & 2.19 & 6564.41 & 6.20  \\
5998.16 & 4.89 & 6303.61 & 27.68 & 6465.29 & 8.10 & 6504.44 & 2.16 & 6564.94 & 2.47  \\
6000.52 & 5.18 & 6306.66 & 20.74 & 6467.00 & 2.75 & 6504.50 & 2.87 & 6564.98 & 2.30  \\
6003.46 & 2.10 & 6307.42 & 22.70 & 6467.14 & 5.23 & 6505.08 & 6.41 & 6565.09 & 14.18  \\
6005.46 & 2.15 & 6310.26 & 2.03 & 6467.59 & 4.57 & 6508.54 & 2.46 & 6569.65 & 2.20  \\
6268.42 & 2.36 & 6310.74 & 15.90 & 6468.44 & 5.69 & 6509.48 & 11.24 & 6569.73 & 4.01  \\
6268.46 & 2.73 & 6311.49 & 16.43 & 6468.75 & 4.17 & 6512.88 & 8.13 & 6572.96 & 14.52  \\
6273.21 & 2.68 & 6315.09 & 10.95 & 6468.82 & 3.20 & 6513.12 & 6.84 & 6575.74 & 22.88  \\
6273.30 & 2.27 & 6315.83 & 11.25 & 6468.84 & 3.08 & 6514.50 & 3.43 & 6580.04 & 2.02  \\
6276.12 & 2.92 & 6317.17 & 5.04 & 6470.23 & 5.43 & 6515.18 & 4.25 & 6581.68 & 7.47  \\
6277.45 & 23.04 & 6318.06 & 4.03 & 6470.51 & 9.69 & 6515.61 & 27.47 & 6584.17 & 2.70  \\
6277.67 & 17.10 & 6318.28 & 2.35 & 6470.87 & 6.62 & 6516.73 & 10.05 & 6584.40 & 3.23  \\
6277.79 & 8.17 & 6319.70 & 7.36 & 6473.34 & 11.43 & 6517.43 & 23.06 & 6584.43 & 3.53  \\
6278.16 & 9.44 & 6320.45 & 6.99 & 6473.48 & 4.90 & 6517.51 & 25.28 & 6586.64 & 2.59  \\
6278.29 & 18.91 & 6320.72 & 2.60 & 6474.05 & 13.43 & 6517.97 & 13.58 & 6587.39 & 8.50  \\
6278.48 & 16.95 & 6320.79 & 4.74 & 6475.00 & 2.52 & 6518.89 & 10.49 & 6587.56 & 4.43  \\
6278.63 & 7.28 & 6322.20 & 2.38 & 6475.92 & 13.86 & 6520.03 & 3.43 & 6587.59 & 3.92  \\
6278.94 & 41.44 & 6324.61 & 6.26 & 6476.07 & 18.40 & 6520.34 & 14.63 & 6595.27 & 4.04  \\
6279.22 & 6.74 & 6324.71 & 3.19 & 6476.68 & 26.54 & 6523.09 & 3.43 & 6600.21 & 6.25  \\
6279.73 & 25.97 & 6324.75 & 3.00 & 6477.88 & 6.04 & 6523.12 & 2.27 & 6603.03 & 3.16  \\
6279.95 & 31.98 & 6325.34 & 3.86 & 6478.20 & 3.65 & 6524.19 & 4.37 & 6606.44 & 2.44  \\
6280.09 & 3.18 & 6329.77 & 2.27 & 6478.36 & 3.04 & 6524.51 & 2.92 & 6606.46 & 2.35  \\
6280.74 & 28.64 & 6330.49 & 2.34 & 6480.06 & 8.64 & 6524.72 & 17.14 & 6613.35 & 2.01  \\
6281.24 & 32.60 & 6332.92 & 3.42 & 6480.35 & 4.81 & 6531.47 & 4.89 & 6613.44 & 3.36  \\
6282.03 & 25.97 & 6343.26 & 4.27 & 6480.93 & 23.10 & 6533.23 & 19.55 & 6835.43 & 2.22  \\        \bottomrule
    \end{tabular}

    \end{threeparttable}
\end{table*}
